# Supplementary material for: Online Estimation and Community Detection of Network Point Processes for Event Streams
Source: arXiv:2009.01742 source file (2023-10-26)
Supplement: Supplementary file 2 [file supp_notation_appendix.tex]

\section{Table of Notation}

Here we provide a table of the key notation used throughout this work.
The specific forms of point processes we consider are given in Section~\ref{Background}.

\begin{table}[h!]
\centering
\begin{tabular}{|p{0.2\textwidth}|p{0.6\textwidth}|}
\hline
 Notation & Meaning  \\
 \hline
 $n$ & The number of nodes in the network.  \\
 $m$ & The current window of online learning.  \\
 $M$ & The number of windows for online learning of currently observed data, which may increase.  \\
 $A$ & The known edge structure, listing node pairs which interact.  \\
 $T$ & The current total observation time.  \\
 $z_i$ & The community assignment of node $i$. \\
 $\lambda$ & The general parameters of a temporal point process. \\
 $\theta$ & The network point process parameters. \\
 $q_i(z)$ & The general mean field variational distribution for the community assignment of the $i$th node.\\
 $dT$ & The length of each of the online optimization windows. \\
 $\mathcal{M}(\tau_i)$ & The multinomial distribution, used as the variational family for $z_i$. \\
 $\tau$ & The parameter of the variational multinomial distribution. \\
 $\pi$ & The group proportion vector.\\
 $S$ & The cumulative history of the network point processes, used for the online estimation.\\
 $K$ & The number of fixed communities in the network. \\
 \hline
\end{tabular}
\end{table}

\newpage
